# Supplementary material for: NVR: Vector Runahead on NPUs for Sparse Memory Access
Source: arXiv:2502.13873 source file (2025-03-17)
Supplement: Supplementary file 1 [file 7_Appendix.tex]

\section{Modelling and Motivation}

\zhenote{Sec.A is a good subsection, but intuitively, I wish to know how it contributes to the paper.}

\vspace{-3pt}
\subsection{Performance Breakdown: Sparsity Accelerate Model}
\vspace{-3pt}
\mionote{this section may be too long?}
\zhenote{Be honest, it is too long.}
Here, we will model the application of sparse properties in model compression and acceleration. We will also analyse why existing systems cannot achieve the ideal sparse acceleration ratio and how to mine the sparse resources of the model to approximate the ideal acceleration ratio. The main focus is on the problem of sparse matrix operations in neural networks, which is representative of most networks \cite{9sparseCNN}.

% \subsubsection{Problem Formulation}
\noindent \textbf{\underline{Problem Formulation}}:
The sparse linear computation at the $h$-th layer of an $L$-hidden-layer fully connected neural network can be defined recursively as follows:
\vspace{-4pt}
\begin{small}
\begin{equation}
\tilde{f}^{(h)}(x) = (W^{(h)} \odot m^{(h)})\tilde{f}^{(h-1)}(x), \quad h = 1, 2, \dots, L
\vspace{-3pt}
\label{eq:eq1}
\end{equation}
\end{small}
where $\tilde{f}^{(h-1)}(x)$ and $\tilde{f}^{(h)}(x)$ represent the input activation (IA) and output activation (OA) of the $h$-th layer respectively. Here, $W^{(h)}$ represents the weight matrix (W), and $m^{(h)}$ is the corresponding sparse mask matrix. 
The operator $\odot$ indicates Hadamard product. %element-wise multiplication.

Consider a weight matrix \( W \in \mathbb{R}^{m \times k} \) and an input activation matrix \( IA \in \mathbb{R}^{k \times n} \). Sparsity ratios are defined for both the row and column dimensions of these matrices: \( s^{(i)}_{W,r} \) and \( s^{(j)}_{W,c} \) for \( W \), and \( s^{(i)}_{IA,r} \) and \( s^{(j)}_{IA,c} \) for \( IA \), where a ratio of 1 indicates a dense matrix. The \( i \)-th row vector of \( W \) and the \( j \)-th column vector of \( IA \), denoted as \( W^T_{i,*} \) and \( IA_{j,*} \) respectively, contribute to the computation of the output activation \( OA \). The sparse mask is generated by independently sampling each element from a Bernoulli distribution with the corresponding probabilities \cite{10Bernoulli}.
% Consider a weight matrix $W \in \mathbb{R}^{m \times k}$ and an input activation matrix $IA \in \mathbb{R}^{k \times n}$. For both matrices, we define sparsity ratios for their row and column dimensions: $s^{(i)}_{W,r}$ and $s^{(j)}_{W,c}$ for matrix $W$, and $s^{(i)}_{IA,r}$ and $s^{(j)}_{IA,c}$ for matrix $IA$, where a ratio of 1 corresponds to a dense matrix. Let $W^T_{i,*}$ and $IA_{j,*}$ denote the $i$-th row vector of $W$ and the $j$-th column vector of $IA$, respectively, which jointly contribute to computing the output activation $OA$.
% % Onthe Neural Tangent Kernel Analysis of Randomly Pruned Neural Networks
% The sparse mask is generated by independently sampling each element from a Bernoulli distribution with these corresponding probabilities \cite{10Bernoulli}. 
According to the Central Limit Theorem, the sparsity distribution can be approximated by a Gaussian distribution.
For instance, the row-wise sparsity distribution of the weight matrix $W$ can be represented as $X_{row}^{(i)} \sim \mathcal{N}(k \cdot s^{(i)}_{W,r}, k \cdot s^{(i)}_{W,r}(1-s^{(i)}_{W,r}))$\cite{11Gaussian}.
%Sparseloop: An Analytical Approach To Sparse Tensor Accelerator Modeling
\zhenote{This section is clear, but is this the true formulation of the problem? It is more like the modeling of the workloads?} \mionote{Right to remind me. I miss the pre-explanation for Systematic Bottleneck Analyze}

% \subsubsection{Ideal Workload and Total Workload}
\noindent \textbf{\underline{Ideal Workload and Total Workload}}:
Input activation $IA$ and weight matrix $W$ can be either independent \cite{} or correlated \cite{} in different neural network architectures \Nnote{mio add cite}. We model their relationship using a two-dimensional Gaussian distribution, where the covariance matrix reduces to diagonal form when they are independent. The expected number of multiplications (workload) is determined by the probability of both elements being non-zero:
% For each element $p_{oa}^{ij}$ in the resulting matrix, the joint probability density function determines its non-zero probability:
\vspace{-7pt}
\begin{small}
\begin{equation}
% \begin{aligned}
% f(x, y) = \frac{1}{2\pi \sigma_x \sigma_y \sqrt{1 - \rho^2}} \exp \left( -\frac{1}{2(1 - \rho^2)} \left[ \frac{(x - \mu_x)^2}{\sigma_x^2} + \frac{(y - \mu_y)^2}{\sigma_y^2} - \frac{2\rho (x - \mu_x)(y - \mu_y)}{\sigma_x \sigma_y} \right] \right)
f(\boldsymbol{X}) = \frac{1}{(2\pi)^{2/d} \left |\Sigma \right |^{1/2} } \exp \left( -\frac{1}{2} (\boldsymbol{X}-\mu)^T \Sigma^{-1} (\boldsymbol{X}-\mu) \right)
% \end{aligned}
\end{equation}
\end{small}
\vspace{-10pt}
\begin{small}
\begin{align*}
    &
\mu = \begin{pmatrix}
         \mu_{IA}^{(i)} \\
         \mu_{W}^{(j)}
        \end{pmatrix},
    &
\Sigma = \begin{bmatrix} 
        {\sigma_{IA}^{(i)}}^2 & \rho^{(ij)} \sigma_{IA}^{(i)} \sigma_{W}^{(j)} \\ 
        \rho^{(ij)} \sigma_{IA}^{(i)} \sigma_{W}^{(j)} & {\sigma_{W}^{(j)}}^2 
        \end{bmatrix},
    &
i \in [0, n], 
j \in [0, m]
    && 
\end{align*}
\end{small}
This joint distribution characterizes the sparsity interaction between $IA$ and $W$. 
Further, the minimum required amount of multiply operations $W_{ideal}$ can be obtained by computing a four-dimensional integral over the sparse matrices' domains $\Omega$, considering only the pairs of non-zero elements.
\vspace{-7pt}
\begin{small}
\begin{equation}
\begin{aligned}
% W_{ideal} &= \int_{0}^{m} \int_{0}^{n} 
% \prod_{i=1}^{d} x_{i} \cdot f\left(\boldsymbol{X}\right) \prod_{i=1}^{d} d x_{i} \\
% &= \prod_{i=1}^{d} s_{i} + \rho \prod_{i=1}^{d} \sigma_{i}
% W_{ideal} &= \sum_{m}^{n}\mathbb{E}[\boldsymbol{X}] = \int_{0}^{n} \int_{0}^{m}  \int_{0}^{k} \int_{0}^{k}
% f\left(\boldsymbol{X}\right) d x_{IA} d x_W \\
W_\mathrm{{ideal}} 
= \sum_{l=0}^{m\times n}\mathbb{E}[\boldsymbol{X_l}] 
= \int_{\Omega} f(\boldsymbol{X}) d\boldsymbol{X}, \Omega = [0,n] \times [0,m] \times [0,k]^2 \\
%&= m \cdot n \cdot (s_{IA} \cdot s_W + \rho \sigma_{IA} \sigma_W)
\end{aligned}
\end{equation}
\end{small}
% However, compared to $W_{total}$, the actual amount of workload, this ideal amount of computation needs to add redundancy. Redundancy comes mainly from the following sources:
However, $W_{total}$, the actual computational workload typically exceeds this ideal case due to various sources of computational redundancy, mainly comes from the following sources:
% \begin{itemize}
% \item[$\bullet$ ] 

1) Sparse alignment: 
Alignment-related redundancy $W_{R}^{align}$ stems from matching non-zero element positions. In practical hardware implementations, rather than pursuing perfect alignment with its associated overhead, many works match the corresponding $IA$ matrix using a sparser matrix $W$\cite{}, introducing additional elements in $IA$. The redundancy is quantified as: $W_{R}^{align} = \sum_{i,j} [P(IA_{i,j} \neq 0) - P(IA_{i,j} \neq 0 \cap W_{i,j} \neq 0)]$ and
$W_{total} = W_{ideal} + W_{R}^{align}$.
%The alignment-related redundant computation $W_{R}^{align}$ arises from the necessity of matching corresponding non-zero element positions. Since achieving perfect alignment may incur additional overhead, we typically opt to match the corresponding $IA$ matrix using matrix $W$ with higher sparsity. This approach introduces additional elements in $IA$. The resulting redundancy can be expressed as: $W_{R}^{align} = \sum_{i,j} [P(IA_{i,j} \neq 0) - P(IA_{i,j} \neq 0 \cap W_{i,j} \neq 0)]$.

% \item[$\bullet$ ] 
2) Sparse skipping and tiling: The construction-related redundant computation $W_{R}^{const}$ arises from hardware limitations in supporting sparse operations. 
Structural computation patterns in hardware may introduce additional redundancy. 
We formulate structural redundancy through constraint functions $\mathcal{C}(X)$.
Through iterative optimization of the function $J(X)$, we obtain the distribution of $X$. The total workload can then be calculated as:
% \end{itemize}
\vspace{-5pt}
\begin{small}
\begin{equation}    
% J(x) = \min_{X}\sum_{m}^{i=0} \left \| X_{i} \left \|_{2} + \sum_{m}^{i=0}\right \| X_{i} -X_{ij}  \right \|_{2} \quad
% \text{s.t.} \quad \mathcal{C}(X)
% \left\{\begin{matrix}
\begin{aligned}
\mathop{\arg\min}\limits_{X}&\mathcal{J}(X)=\sum_{i=0}^{{tile}} \|\hat{x}_{i}\|_{2} + \sum_{i=0}^{{element}}\|\hat{x}_{i} - x_{sub}\|_{2}\\
 % &J(X) = \lambda_1\sum_{i=0}^{m} \|X_{i}\|_{2} + \lambda_2\sum_{i=0}^{m}\|X_{i} -X_{ij}\|_{2}\\
 & s.t. \quad \mathcal{C}(X) \in \{c_{row}(X), c_{col}(X), \cdots\}\\
% &W_{total} = \sum_{X} J^*(X) \text{ where } J^*(X) = \arg\min_{X} J(X) \text{ s.t. } \mathcal{C}(X)
\end{aligned}
% \end{matrix}\right.
\end{equation}
\end{small}
% $$
% W_{total} = \sum_{X} J^*(X) \text{ where } J^*(X) = \arg\min_{X} J(X) \text{ s.t. } \mathcal{C}(X)
% $$
% where $J^*(X)$ represents the optimal solution under the constraint $\mathcal{C}(X)$, obtained through iterative optimization.
where $\hat{x}_{i}$ denotes the leading element of each tile and $x_{sub}$ represents the sub-element within the tile. Through optimization, we obtain the optimal distribution of $X$, with $W_{total}$ representing its final size.

\noindent \textbf{\underline{Execution Time Calculation}}: The total execution time consists of two main components: computation time $T_{comp}=\frac{W_{total}}{MAC}$ and I/O time $T_{IO}$. $MAC$ denotes the peak computing capability of the hardware platform. 
% \subsubsection{Execution Time}
% \begin{small}
% \begin{equation}
% T_{comp} = \frac{W_{total}}{MAC}
% \end{equation}
% \end{small}
\vspace{-5pt}
\begin{small}
\begin{equation}
\label{eq:eq3}
\left\{   
\begin{aligned}
& T_{IO} = \frac{W_{mvin} + W_{mvout}}{BW} + G(\boldsymbol{X}, BW) \\
& G(X) = \mathbbm{1}(prefetch)\frac{W_{prefetch}}{BW} + \sum_{i=1}^{2}\mathbbm{1}(l_i)t_{l_i}f^{(l_i)}_{miss}(\boldsymbol{X})\\
% & G(\boldsymbol{X} , BW, c_i)  = \\
% & \quad \left\{   
% \begin{aligned}
% & \frac{W^{l1miss}_{prefetch}}{BW} + t_{l1} f^{l1}_{miss}(\boldsymbol{X})+ t_{l2} f^{l2}_{miss}(\boldsymbol{X}), c_0 \neq 0\\
% & \frac{W_{prefetch}}{BW} + f^{l2}_{miss}(\boldsymbol{X}), c_1 \neq 0 \\
% & f^{l2}_{miss}(\boldsymbol{X}), c_2 \neq 0  \\
% \end{aligned}
% \right. \\
% &f_{miss}=p_{k}(i-1) \frac{1-\sum_{t=1}^{K} \alpha_{t} b_{t}(i-2)-\alpha_{k}}{1-\sum_{t=1}^{K} \alpha_{t} b_{t}(i-1)}, i \subseteq[2, M]\\
\end{aligned}
\right.
\vspace{-5pt}
\end{equation}
\end{small}
The I/O time model captures the memory hierarchy effects through several components: 
(1) data movement costs $W_{mvin}$ and $W_{mvout}$, 
(2) cache miss penalties modelled by $f_{miss}$, a predictive model provided by\cite{} \Nnote{mio add cite},
% and
(3) prefetch overhead. 
The indicator function $\mathbbm{1}(*)$ determines each system model is whether active (l1, l2, prefetch).

% \subsubsection{Systematic Speedup and Scalability}
\noindent \textbf{\underline{Systematic Bottleneck Analyze}}:
Considering Gustafson's Law and the Roofline model, we can analyze the system's performance bottlenecks and actual acceleration curve. The effective speedup $S$ can be expressed as: $S=\min(T_{comp}, T_{IO})$

This framework guides performance optimization for sparse DNN workloads across diverse hardware scenarios. Fig. \ref{fig:fig2} illustrates these characteristics, where red dots indicate the operational points of different sparse workloads. The results show that I/O is the current workload's bottleneck, which can be effectively mitigated through prefetching.
\zhenote{Hi, could you please summarize how do the above paragraphs contribute to the whole story?}

%It can be said that the more effectively we leverage a model's sparse characteristics, the closer we approach actual \textbf{S}parse storage, \textbf{S}parse IO, and \textbf{S}parse compute, which we collectively refer to as "\textbf{3S}". In this scenario, our actual speedup can increasingly approach the theoretical speedup brought about by sparsity, which is essentially the sparsity ratio.
